# Supplementary material for: Non-affinity and fluid-coupled viscoelastic plateau for immersed fiber networks
Source: arXiv:1908.07768 source file (2019-11-13)
Supplement: Supplementary file 1 [file suppInf_resubOct2019.pdf]

**Supplementary Information for 'Non-affinity and fluid-coupled viscoelastic plateau for immersed fiber networks,' D.A. Head and C. Storm.**

This supplementary information includes:

- Page 1: Fluid contribution to the complex modulus *(calculation)*.
- Page 2: Fig. S1 *(numerical: evaluation of incompressibility)*.
- Page 3: Fig. S2 *(numerical: robustness with respect to fluid mesh size)*.
- Page 4: Fig. S3 *(result: $G^*(\omega)$ for a non-rigid network)*.
- Page 5: Fig. S4 *(result: frequencies extracted from the double Maxwell fit)*.

## 1. Fluid contribution to the complex modulus

The net contribution by the fluid to the shear stress $\sigma_{xy}$ can be evaluated by taking the average of the local shear stress $\eta\partial_y v_x$, where $v_x$ is the $x$-component of the fluid velocity. For definiteness, assume the box is rectangular with dimensions $(X, Y)$ as in the main text. Then

$$\sigma_{xy}^{\text{fluid}}(t) = \eta\langle\partial_y v_x(x,y,t)\rangle \tag{S1}$$

$$= \frac{\eta}{XY}\int_0^X \mathrm{d}x \int_0^Y \mathrm{d}y\, \partial_y v_x(x,y,t) \tag{S2}$$

$$= \frac{\eta}{XY}\int_0^X \mathrm{d}x\, \left[v_x(x,y,t)\right]_{y=0}^{y=Y} \quad . \tag{S3}$$

Since the fluid velocity at the boundaries $y = 0$ and $y = Y$ are imposed by the external driving and therefore known and homogeneous, the integrand $[v_x(x,y,t)]_{y=0}^{y=Y}$ can be replaced by $i\omega\gamma Y e^{i\omega t}$, using the same complex notation as the main text. This simplifies (S3) to

$$\sigma_{xy}^{\text{fluid}}(t) = \frac{i\omega\gamma\eta}{X}\int_0^X \mathrm{d}x\, e^{i\omega t} = i\omega\gamma\eta e^{i\omega t}\,, \tag{S4}$$

corresponding to a contribution to $G^*(\omega)$ of $i\omega\eta$ as given in equation (4) in the main text.

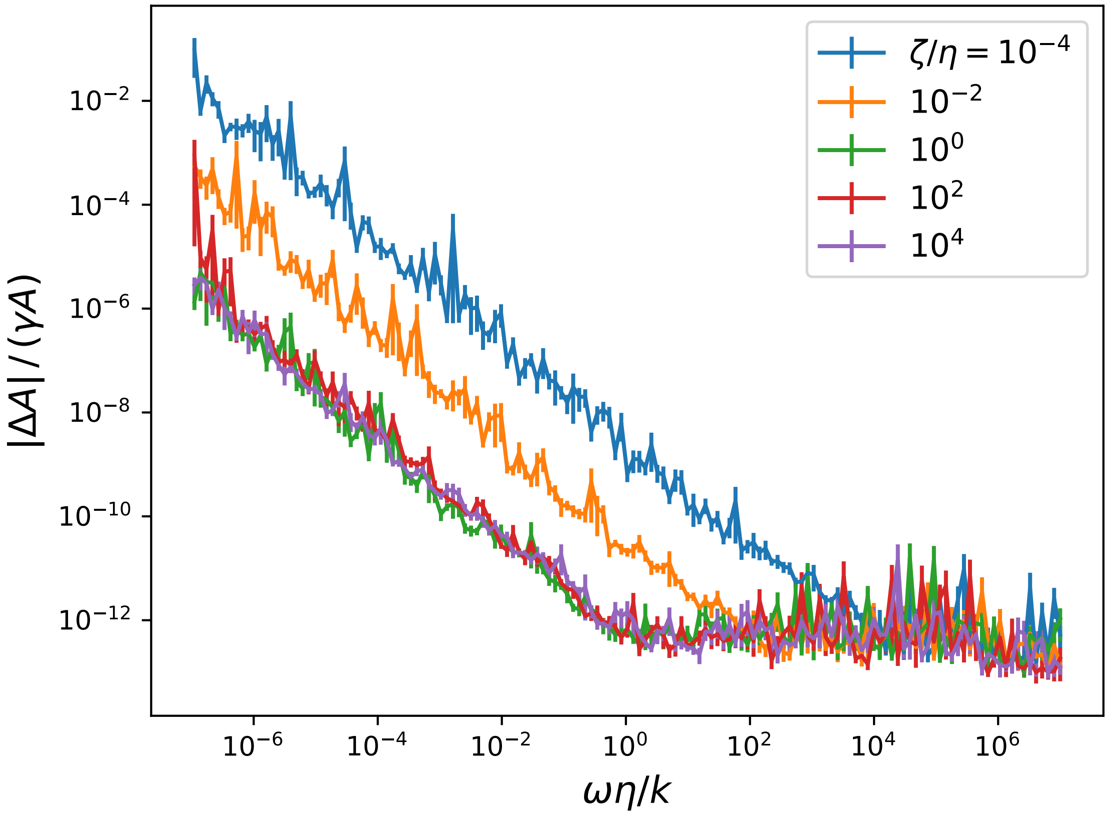


Figure S1: Relative change in fluid mesh area with frequency for the $\zeta$ given in the legend. $|\Delta A|$ is the summed absolute change in area of each velocity mesh rectangle, using a linearised expression based on the $v_{ij}$ at each corner node, and $A$ is the initial area.

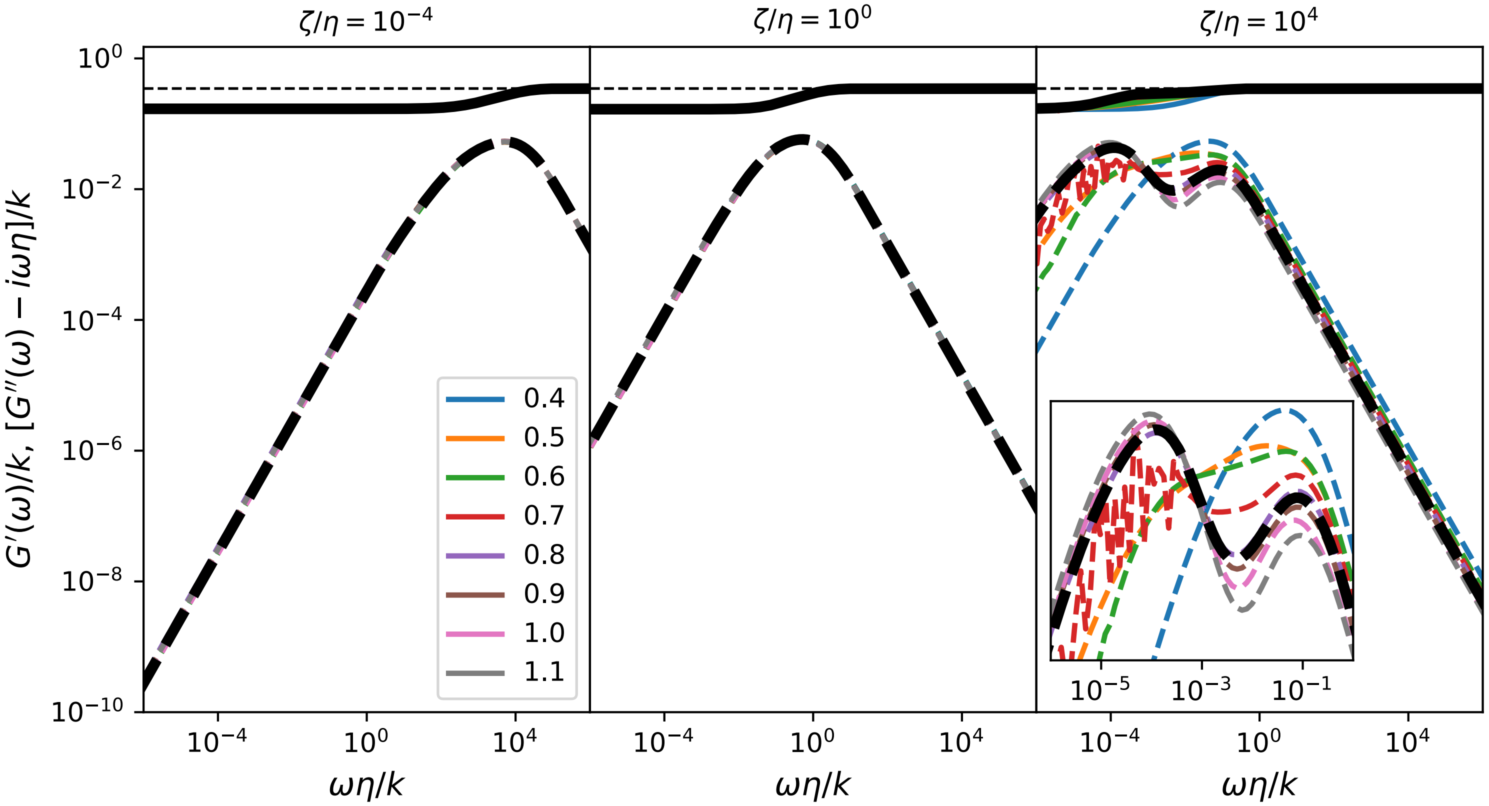


Figure S2: $G'(\omega)$ (solid lines) and the network contribution to $G''(\omega)$ (dashed lines) for $p = 0.8$ and varying cell size for the fluid meshes relative to the natural spring length $\ell_0$, as indicated in the legend in the left-hand panel. The coupling coefficient varies from left to right as $\zeta/\eta - 10^{-4}$, 1 and $10^4$. The thick bold lines correspond to the value 0.83 used elsewhere. In all panels the horizontal dashed line gives the affine prediction $G_0 = pk\sqrt{3/4}$. The inset in the right-hand panel shows $[G''(\omega) - i\omega\eta]/k$ in the region of greatest variation. Although quantitative variation with fluid mesh size is evident for the highest coupling coefficient $\zeta = 10^4\eta$, qualitative deviations only arise for small mesh sizes less than 0.7 times $\ell_0$. This is presumably an artefact of coupling only at network nodes, which permits fluid cells uncoupled to the network in between nodes when the fluid mesh size is sufficiently small.

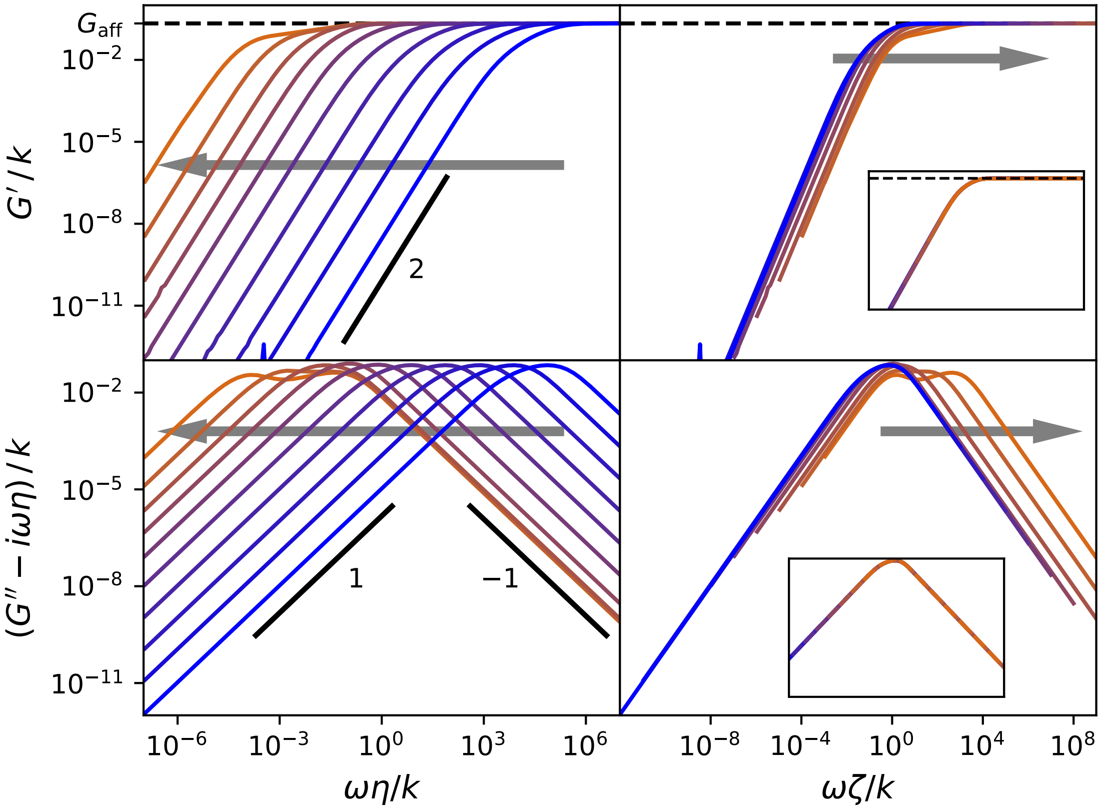


Figure S3: $G'(\omega)$ (top panels) and the network contribution to $G''(\omega)$ (lower panels) for $p = 0.5$, with large arrows showing different $\zeta/\eta$ increasing from $10^{-5}$ (dark curves) to $10^{4}$ (light curves) in factors of ten (note this range slightly differs from the $p = 0.8$ plot in the main text). The insets show data over the same ranges without hydrodynamic interactions. The horizontal dashed line in the upper panels show the affine prediction $G_{\rm aff} = pk\sqrt{3}/4$. The line segments in the left-hand panels have the denoted slope. Each line is averaged over 10 networks with $100 \times 100$ nodes.

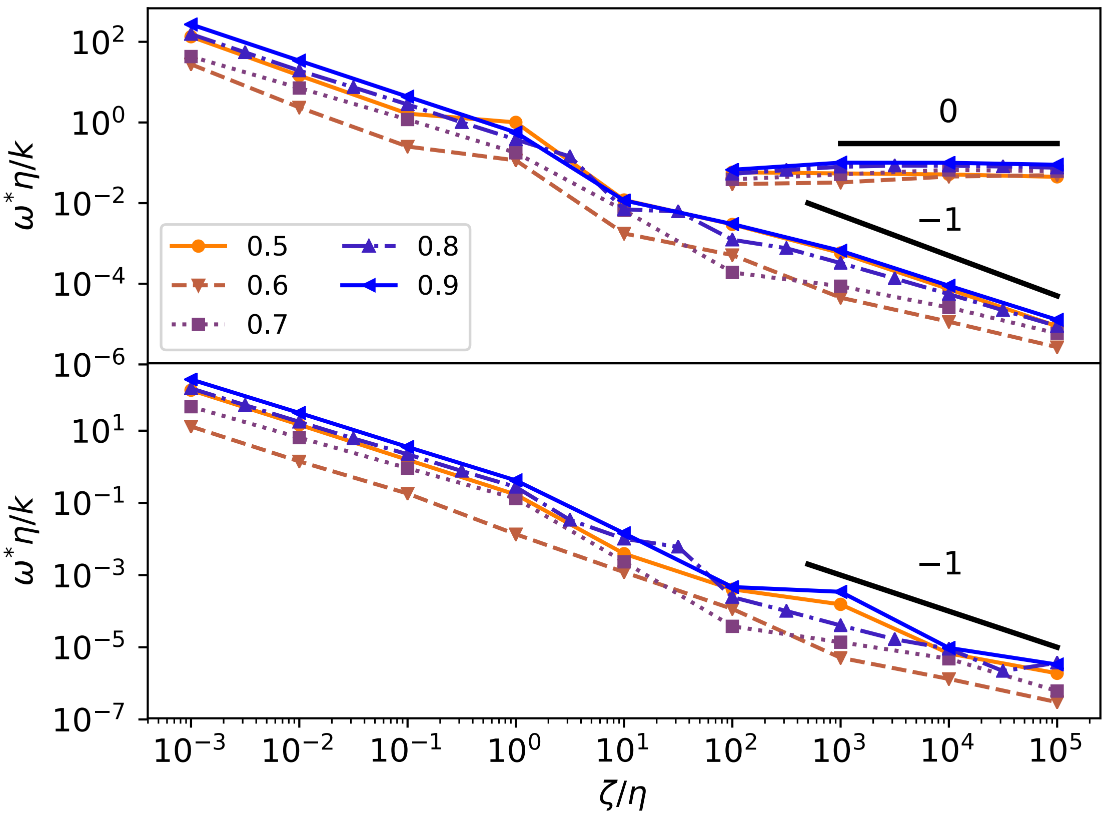


Figure S4: Frequencies $\omega^*$ extracted from the double-Maxwell predictions for $G'(\omega)$ and $G''(\omega)$, (5) and (6) in the main text, for the bond dilutions $p$ given in the legend. When there is only one $\omega^*$, it corresponds to a fitted value of the effective drag coefficient, *i.e.* $\omega^* = k/\zeta^{\text{eff}}$, as given in the main text. When there is a second, then the higher $\omega^*$ corresponds to $\omega^* = k/\eta^{\text{eff}}$ with $\eta^{\text{eff}}$ an effective viscosity. Note that the $\zeta$, $\eta$ and $k$ in the figure axes labels are the known input values for these parameters, so the fits demonstrate that $\zeta \approx \zeta^{\text{eff}}$ and $\eta \approx \eta^{\text{eff}}$. The upper panel is with hydrodynamic interactions, the lower without, and the black line segments have the given slope. Note there is no signature of the rigidity transition $p = p_{\text{c}} \approx 0.66$, as this primarily affects the low-frequency tails and not the location of the peak(s).
